# Supplementary material for: Bayesian Spline Learning for Equation Discovery of Nonlinear Dynamics with Quantified Uncertainty
Source: arXiv:2210.08095 source file (2022-10-14)

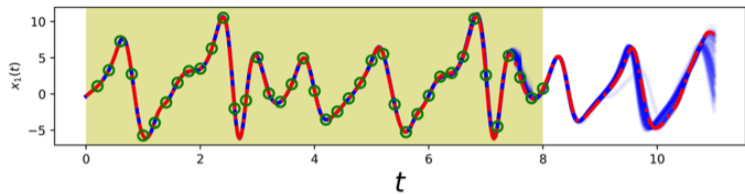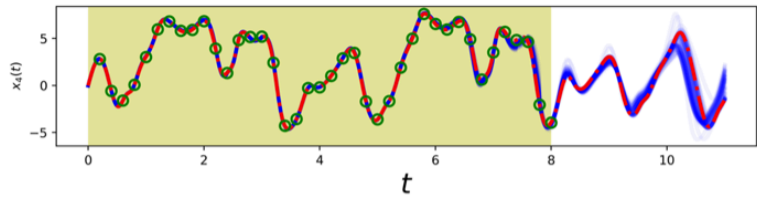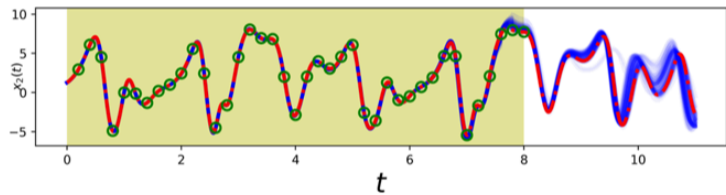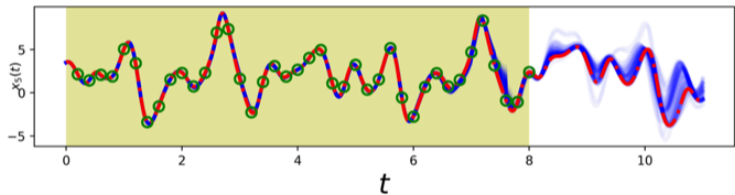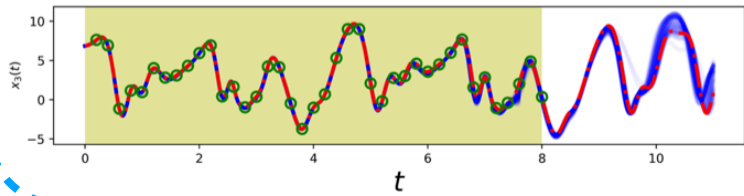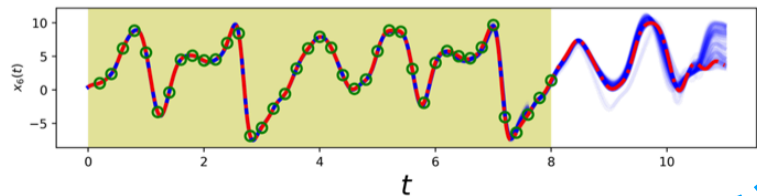

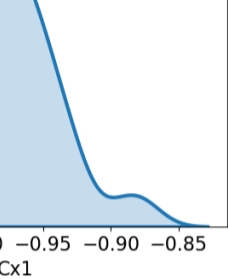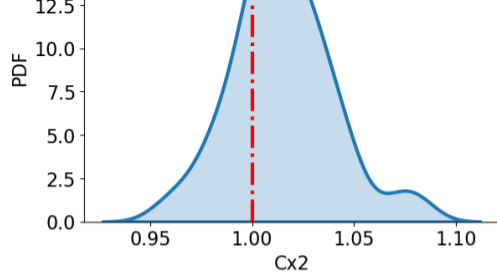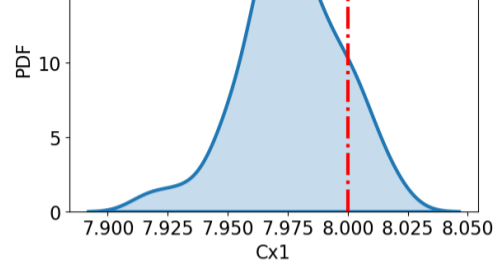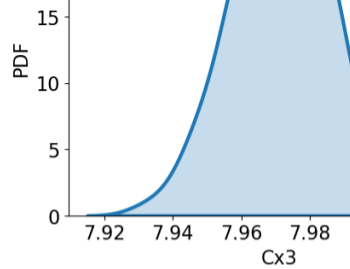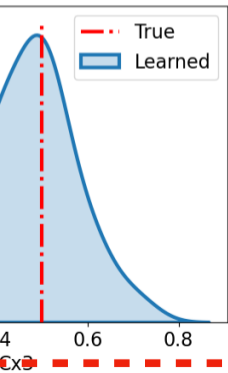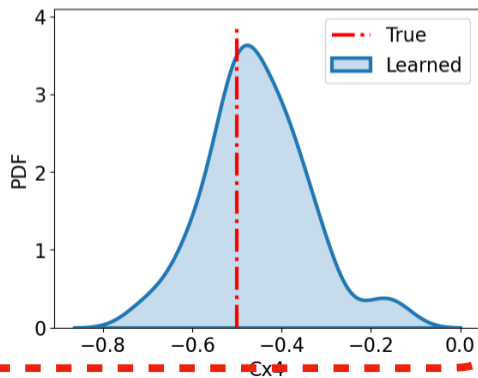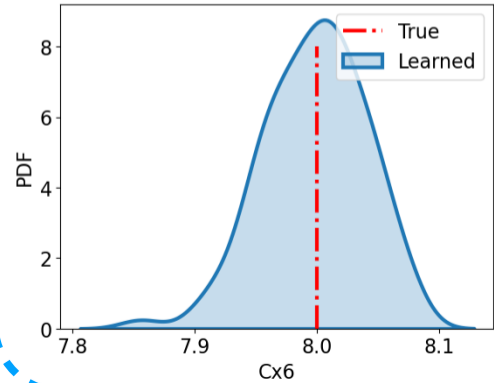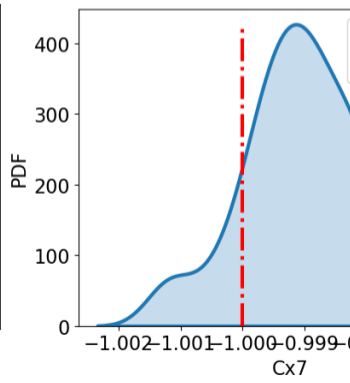

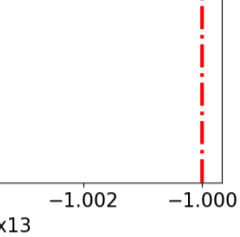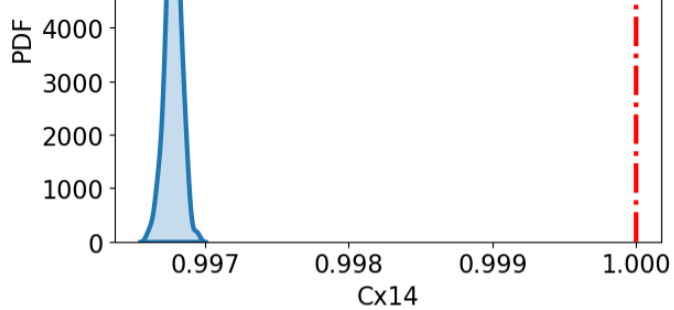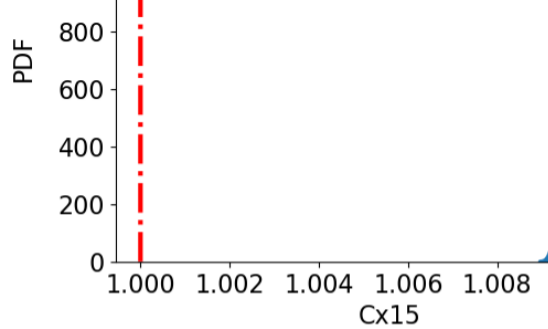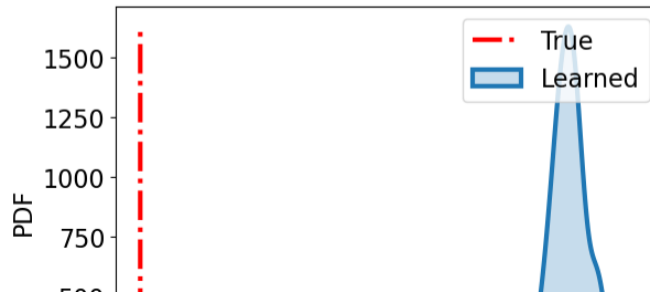

Spine Learning

Bayesian ADO  
Training

UQ

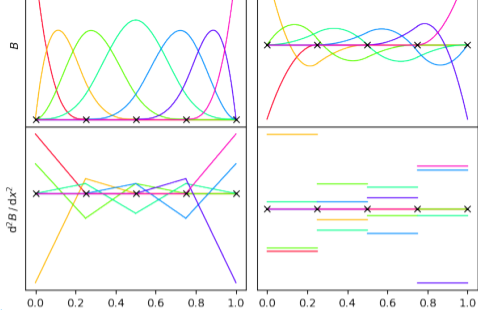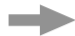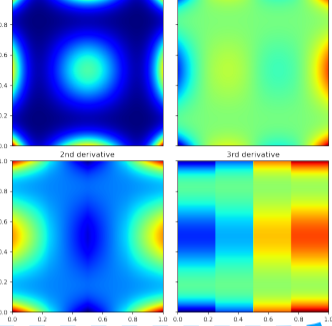

$W^*, B, P$

EnKF

Learning Rate

$$L \propto \text{priors} + (\hat{\mathbf{U}} - N_m \boldsymbol{\theta})^T \mathbf{B}^{-1} (\hat{\mathbf{U}} - N_m \boldsymbol{\theta}) + (\dot{N}_c \boldsymbol{\theta} - \Phi(N_c \boldsymbol{\theta}) W^*)^T \mathbf{P}^{-1} (\dot{N}_c \boldsymbol{\theta} - \Phi(N_c \boldsymbol{\theta}) W^*)$$

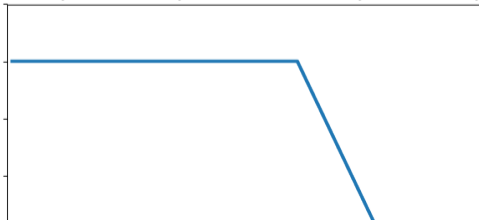

$\Phi(\boldsymbol{\theta}), \dot{\mathbf{U}}(\boldsymbol{\theta}), P$

$$W^*_{n \times d} = W_{m \times d}$$

$$\frac{du_1}{dt} \quad \frac{du_2}{dt}$$

=

$1 \quad u_1 \quad u_2 \quad u_2^3 \quad w_1 w_2$

$W$

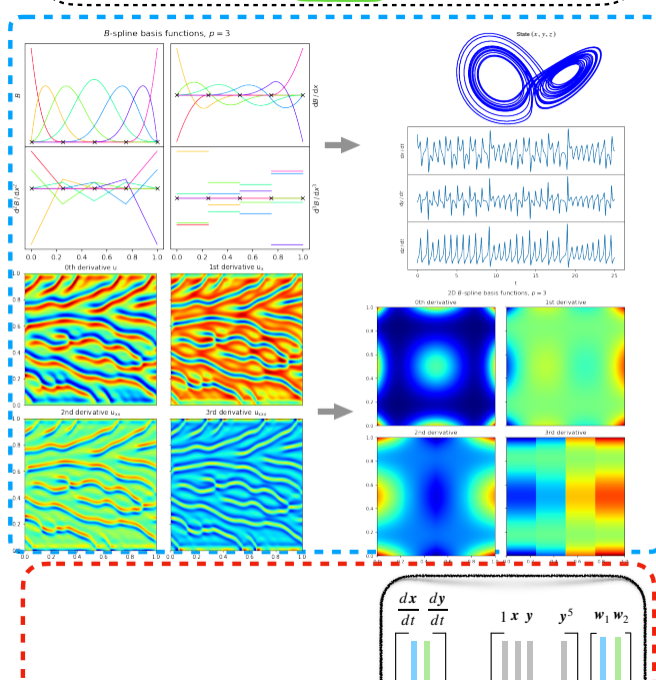

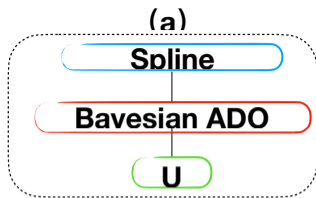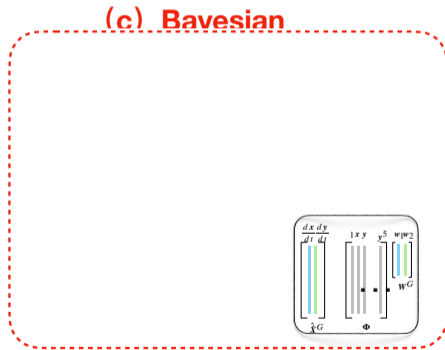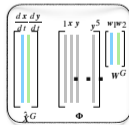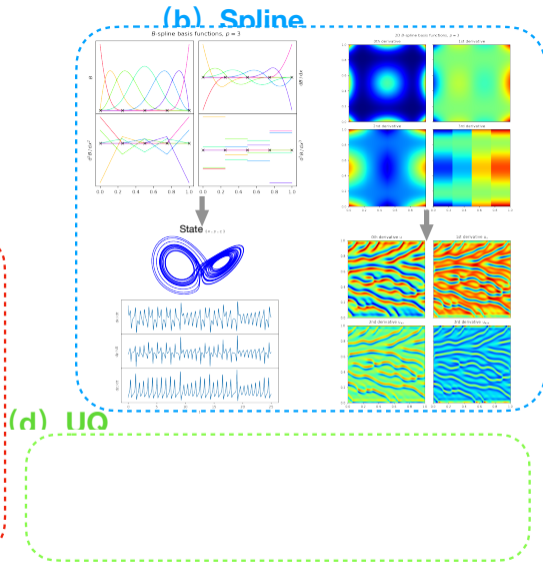

(d) UQ

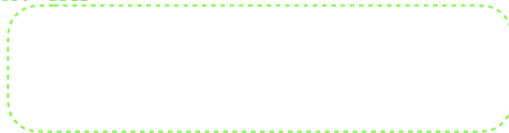

Supplement: Supplementary file 1 [file crop_UQODE.pdf]
